# Supplementary material for: Top-down and bottom-up excursions beyond the Standard Model: The example of left-right symmetries in supersymmetry
Source: arXiv:1404.4564 source file (2014-04-17)
Supplement: Supplementary file 1 [file rges_lrsusy.tex]

\subsection{Renormalization group equations}
\begingroup
\allowdisplaybreaks
% [inline block 0: 1 envs, 207342 chars -> math_tex | \begin{align} \n ...]
%
\endgroup
